# Supplementary material for: Towards Optimal Use of Exception Handling Information for Function Detection
Source: arXiv:2104.03168 source file (2021-04-07)
Supplement: Supplementary file 1 [file appendix.tex]

\iffalse
\section{Benchmark Binaries Used in Our Studies}
\label{sec:benchmark}
We used two groups of benchmark binaries in our studies, one from the wild and one being self-built. The binaries from the wild are summarized in Table~\ref{tab:comtools} and the self-built binaries are summarized in Table~\ref{tab:dataset}.






\section{Implementation of \tool}
\label{app:impl}

We have implemented the optimal strategies of using FDEs as a tool called \tool, on top of \dyninst-10.1.0 with about 2,000 lines of C++ code. \tool takes a stripped binary as input and outputs the list of function starts. In this section, we cover the important implementation details. 

\subsection{Parsing \ehf} To obtain the FDEs and CFIs inside each FDE, we reuse the Libdwarf library (version 20200114) to parse the \ehf section. Recall that \tool needs to determine the stack height based on CFIs. To do this, we re-use the \texttt{dwarf\_get\_fde\_info\_for\_all\_regs3} API from Libdwarf to obtain the relation between \texttt{rsp} and CFA and then calculate the stack height. 

\begin{figure}[!t]
  \centering
\begin{lstlisting}[language={[x86masm]Assembler},basicstyle={\footnotesize\ttfamily},numberstyle=\scriptsize,deletekeywords={df},xleftmargin=5mm]
mov edx,eax ; creating an implicit alias
and al,0xf
and edx,0xf
cmp al,0x4
ja fdc152
jmp QWORD PTR [rdx+0x15eb410*8]
\end{lstlisting}
\caption{A jump table in {\tt MySqld} compiled with Clang-6.0.0. \dyninst cannot correctly find the value range of the index (\texttt{rdx} in line 6), because it does recognize the ``implicit'' alias between \texttt{al} (at line 2 and 4) and \texttt{rdx} (at line 6) and hence, misses capturing the constraint enforced to the index at line 4. \label{lst:alias_jmptbl}}
\end{figure}

\subsection{Recursive Disassembly} 
\label{subsec:impl:disa}
Given an address that we consider as a function start, we re-use the \texttt{parse} API from the \texttt{ParseAPI::CodeObject} class in \dyninst to do recursive disassembly, with the built-in tail call detection disabled. We also extended the list of non-returning library functions used by \dyninst, resulting in a final list shown in Table~\ref{tab:nonret_funcs}. To determine the first argument passed to {\tt error} and {\tt error\_at\_line}, we need to do backward slicing, for which we re-use the \texttt{backwardSlice} API from the \texttt{Slicer} class in \dyninst. Finally, we found three defects in \dyninst's implementation of handling jump tables. First, it cannot recognize a special type of alias when performing VSA. An example of such alias is shown in Fig.~\ref{lst:alias_jmptbl} and we fixed it accordingly. Second, when it performs backward slicing, it restrict the scope to be 50 assignments, which can lead to many errors. We removed this restriction. Finally, it wrongly assumes the \texttt{.data} section is read only. We fixed this by removing the read-only assumption.

%In particular, for {\tt error} and {\tt error\_at\_line}, they are non-returning only when their first argument is non-zero. To determine the value of the first argument, we run backward slices using the argument as source and examine whether the argument is always propagated from a constant. If so, we set the returning status of the function in accordance to the constant value. Otherwise, we consider the function returns. 

\subsection{Error Checking} While running recursive disassembly from a potential pointer, \tool determines the correctness of disassembly by checking four types of errors. We describe how we implemented each of them as follows: (i) we re-use the \texttt{isLegalInsn} API from \dyninst to check the legitimacy of each instruction; (ii) we examine each basic block to check if it runs into already-disassembled instructions; (iii) we examine each basic block to check if it runs into the middle of already-detected functions; (iv) we examine the calling conventions by checking if a non-argument register is always initialized before use. To do this, we rely on liveness analysis, re-using the {\tt LivenessAnalysis} class provided by \dyninst. Specifically, if a non-argument register alive at the function start is still alive at its uses, we consider it violates the calling conventions. Note that we prevent \dyninst from considering the use of registers in \texttt{push} instructions (\eg \texttt{push rbx}) since such instructions can be saving callee-saved registers. 

%Eh-disassembler utilize the starting and ending function address in FDE record in eh\_frame. First round recursive disassembling begin from the starting function address. Eh-disassembler also run cross-reference analysis to identify those functions that can not be reached during first round recursive disassembling. In reference disassembling, corss-reference targets collected from linearly scanning code and data regions will be used as start address for recursive disassembly. If the recursive disassembly does not run into errors, eh-disassembler consider the function pointer refers to a valid function and collect the functions detected by the recursive disassembly. 

\section{Interesting Cases}
\label{app:cases}


\begin{figure}[htb!]
  \centering
\begin{lstlisting}[basicstyle={\footnotesize\ttfamily},numberstyle=\scriptsize,linewidth=0.9\columnwidth,xleftmargin=5mm]
virtual ~Sized_dwarf_line_info(){ 
    if (this->buffer_start_ != NULL) 
        delete[] this->buffer_start_;
}
\end{lstlisting}
  \caption{An example of destructor function without symbol.}
  \label{fig:destructor}
\end{figure}


\begin{figure}[htb!]
    \centering
\begin{lstlisting}[language={[x86masm]Assembler},basicstyle={\footnotesize\ttfamily},numberstyle=\scriptsize,xleftmargin=5mm,deletekeywords={df,}]
; function start
__bn_postx4x_internal: ; symbol without type
	mov	8*0($nptr),%r12
	mov	%rcx,%r10		# -$num
	mov	%rcx,%r9		# -$num
	neg	%rax
	sar	\$3+2,%rcx
	#lea	48+8(%rsp,%r9),$tptr
	movq	%xmm1,$rptr		# restore $rptr
	movq	%xmm1,$aptr		# prepare for back-to-back call
	dec	%r12			# so that after 'not' we get -n[0]
	mov	8*1($nptr),%r13
	xor	%r8,%r8
	mov	8*2($nptr),%r14
	mov	8*3($nptr),%r15
	jmp	.Lsqrx4x_sub_entry
; function end
\end{lstlisting}
  \caption{An assembly function without symbol type.}
  \label{fig:assfunc}
\end{figure}


\begin{figure}[htb!]
    \centering
\begin{lstlisting}[language={[x86masm]Assembler},basicstyle={\footnotesize\ttfamily},numberstyle=\scriptsize,xleftmargin=5mm,deletekeywords={df,}]
; function start
00000000004037c0 <ucase>:
  4037c0:   jmp    4037db; considered as a thunk function
  4037c2:   nopw   0x0(%rax,%rax,1)
  4037c8:   lea    -0x61(%rax),%ecx
  4037cb:   lea    -0x20(%rax),%edx
  4037ce:   cmp    $0x1a,%cl
  4037d1:   cmovb  %edx,%eax
  4037d4:   add    $0x1,%rdi
  4037d8:   mov    %al,-0x1(%rdi)
; wrong function start  
  4037db:   movzbl (%rdi),%eax; false positive
  4037de:   test   %al,%al
  4037e0:   jne    4037c8 
  4037e2:   retq
  4037e3:   nopl   (%rax)
  4037e6:   nopw   %cs:0x0(%rax,%rax,1)
; function end
\end{lstlisting}
  \caption{A wrong thunk function detected by \ghidra from Sphinx\_livepretend (compiled with GCC and O2).}
  \label{fig:thunkfunc}
\end{figure}

\begin{figure}[htb!]
    \centering
\begin{lstlisting}[language={[x86masm]Assembler},basicstyle={\footnotesize\ttfamily},numberstyle=\scriptsize,xleftmargin=5mm,deletekeywords={df,}]
; function start 1
00000000004d6aa0 <func1>:
  4d6aa0:   mov	$0x1,%edx; a function start
  4d6aa5:   jmp	4d6aa7; a jump to the next function
; function end 1
; function start 2
00000000004d6aa7 <func2>:
  4d6aa7:   push   %rbp; another function start
  4d6aa8:   push   %r14
  4d6aaa:   push   %rbx
  4d6aab:   sub	$0x10,%rsp
  4d6aaf:   mov	%edx,%r14d
  4d6ab2:   mov	%esi,%ebp
  4d6ab4:   test   %rdi,%rdi
  4d6ab7:   je 	4d6ae6
  4d6ab9:   cmpb   $0x0,(%rdi)
  4d6abc:   je 	4d6ae6
  4d6abe:   xor	%edx,%edx
  ...
 ; function end 2
\end{lstlisting}
  \caption{An example from Busybox compiled with Clang and Os. \angr wrongly merged {\tt func2} to {\tt func1} because the two functions are connected via the {\tt jmp} at {\tt 0x4d6aa5} and the two functions happen to be neighbors.}
  \label{fig:angrmerge}
\end{figure}


\begin{figure}[htb!]
    \centering
\begin{lstlisting}[language={[x86masm]Assembler},basicstyle={\footnotesize\ttfamily},numberstyle=\scriptsize,xleftmargin=5mm,deletekeywords={df,}]
; function start
00000000006688f0 <dump_enabled_p>:
  6688f0:   mov %edi,%edi; detected as padding
  6688f2:   lea (%rdi,%rdi,2),%rax; considered as a new function start
  6688f6:   mov 0x7c8954(,%rax,8),%eax
  6688fd:   retq
  6688fe:   xchg   %ax,%ax
; function end
\end{lstlisting}
  \caption{An example from Objdump compiled with GCC and Ofast. \angr considers the first instruction at {\tt 6688f0} as padding and further considers the second instruction at {\tt 6688f2} as a new function start.}
  \label{fig:angrpaddingfp}
\end{figure}

\section{Non-returning Library Functions Used by \tool.}
\label{sec:non-return:func}

% \section{Non-ret functions in libs}
\newcommand{\tabincell}[2]{\begin{tabular}{@{}#1@{}}#2\end{tabular}}


\begin{table}[H]
%\setlength\tabcolsep{4pt}
  \centering
  \caption{Non-returning library functions used by \tool.}
  \label{tab:nonret_funcs}
  \scriptsize
%   \scalebox{1.0}{
  \begin{tabular}{c|c}
  \toprule[0.5pt]
  \toprule[0.5pt]
  { Unconditional} & 
     \tabincell{c}{\_\_GI\_\_\_assert\_fail, \_Exit, \_\_GI\_\_\_chk\_fail, \\ \_\_GI\_\_\_assert\_perror\_fail, \_\_GI\_\_\_fortify\_fail, \\
 \_\_GI\_\_\_libc\_dynarray\_at\_failure, \_\_GI\_\_\_libc\_fatal, \\ \_\_GI\_\_dl\_signal\_error, \_\_GI\_\_exit, \_\_GI\_abort, \\
 \_\_GI\_exit, \_\_GI\_verr, \_\_GI\_verrx, \_\_assert, \\ \_\_assert\_fail, \_\_assert\_fail\_base, \_\_assert\_perror\_fail, \\ 
 \_\_chk\_fail, \_\_fortify\_fail, \_\_libc\_dynarray\_at\_failure, \\
 \_\_libc\_fatal, \_\_libc\_main, \_\_libc\_siglongjmp, \\ \_\_libc\_start\_main, \_\_run\_exit\_handlers,\\
 \_\_stack\_chk\_fail, \_\_stack\_chk\_fail\_local, \\ \_dl\_signal\_error, 
 \_dl\_start, \_exit, \_longjmp, abort, err, \\
 errx, exit, fatal\_error, longjmp, mabort, \\
 malloc\_printerr, print\_and\_abort, siglongjmp, \\
 svctcp\_rendezvous\_abort, svcunix\_rendezvous\_abort\\
 verr, verrx, \_\_GI\_\_\_pthread\_unwind, \\
 \_\_GI\_\_\_pthread\_unwind\_next, \_\_nptl\_main, \\
 \_\_pthread\_unwind, \_\_pthread\_unwind\_next \\
 longjmp\_alias, longjmp\_compat, pthread\_exit, \\
 siglongjmp\_alias, start\_thread, thrd\_exit, \\
 \_ZN10\_\_cxxabiv111\_\_terminateEPFvvE, \\
 \_ZN10\_\_cxxabiv112\_\_unexpectedEPFvvE, \\
 \_ZN9\_\_gnu\_cxx26\_\_throw\_insufficient\_spaceEPKcS1\_, \\
 \_ZNK11\_\_gnu\_debug16\_Error\_formatter8\_M\_errorEv, \\
 \_ZSt10unexpectedv, \_ZSt17\_\_throw\_bad\_allocv, \\
 \_ZSt17rethrow\_exceptionNSt15\_\_\- \\
 exception\_ptr13exception\_ptrE \\
 \_ZSt18\_\_throw\_bad\_typeidv, \\
 \_ZSt19\_\_throw\_ios\_failurePKc, \\
 \_ZSt19\_\_throw\_ios\_failurePKci, \\ \_ZSt19\_\_throw\_logic\_errorPKc \\
 \_ZSt19\_\_throw\_range\_errorPKc, \\ \_ZSt20\_\_throw\_domain\_errorPKc, \\
 \_ZSt20\_\_throw\_future\_errori, \\ \_ZSt20\_\_throw\_length\_errorPKc, \\
 \_ZSt20\_\_throw\_out\_of\_rangePKc, \\
 \_ZSt20\_\_throw\_system\_errori, \\
 \_ZSt21\_\_throw\_bad\_exceptionv, \\
 \_ZSt21\_\_throw\_runtime\_errorPKc, \\
 \_ZSt22\_\_throw\_overflow\_errorPKc, \\
 \_ZSt23\_\_throw\_underflow\_errorPKc, \\
 \_ZSt24\_\_throw\_invalid\_argumentPKc, \\
 \_ZSt24\_\_throw\_out\_of\_range\_fmtPKcz, \\
 \_ZSt25\_\_throw\_bad\_function\_callv, \\
 \_ZSt9terminatev, \_\_cxa\_bad\_cast, \_\_cxa\_bad\_typeid, \\ \_\_cxa\_call\_unexpected, \_\_cxa\_deleted\_virtual \\
 \_\_cxa\_pure\_virtual, \_\_cxa\_rethrow, \_\_cxa\_throw, \\ \_\_cxa\_throw\_bad\_array\_new\_length, 
 \\ \_\_error\_at\_line\_noreturn, \_\_error\_noreturn,
 \\ \_\_longjmp\_chk, quick\_exit, \_\_f90\_stop, \\ 
  ExitProcess, \_Unwind\_Resume, \_\_longjmp, \\ fancy\_abort,, \_gfortran\_abort, \_gfortran\_exit\_i8, \\ \_gfortran\_exit\_i4, for\_stop\_core, \_\_sys\_exit, \\
 \_gfortran\_error\_stop\_numeric, \\ \_gfortran\_error\_stop\_string, \\
 \_gfortran\_os\_error, \_gfortran\_runtime\_error, \\
 \_gfortran\_runtime\_error\_at, \_gfortran\_stop\_numeric, \\
 \_gfortran\_stop\_string, \_gfortrani\_exit\_error, \\
 \_gfortrani\_internal\_error, \_gfortrani\_os\_error, \\
 \_gfortrani\_runtime\_error, \_gfortrani\_runtime\_error\_at, \\ \_gfortrani\_sys\_abort, \\
 xexit, \_bfd\_abort, \_Z8V8\_FatalPKciS0\_z} \\ \hline
  {Conditional} & error, error\_at\_line \\
    
    \toprule[0.5pt]
    \toprule[0.5pt]
  \end{tabular}
%   }
\end{table}

\fi
